# Supplementary material for: e-ViL: A Dataset and Benchmark for Natural Language Explanations in Vision-Language Tasks
Source: arXiv:2105.03761 source file (2021-08-18)
Supplement: Supplementary file 1 [file notes.tex]

\section{human }

\subsection{e-SNLI-VE improve measures}

detecting fn: In terms of detecting false neutrals, our method has a recall of 0.43 and a precision of 0.61.

 Marasovic et al.~\cite{marasovic_natural_2020} also assessed the raw dataset and found that 81\% and 77\% of explanations are plausible (for a sample of 250 contradiction and entailment pairs).

\section{MTurk eval}

By taking the same sample of 300 examples for each dataset and not only evaluating those that were predicted correctly (as done in xxPark), 
Previous work xxCite has coniditioned (xxVerify) the explanations on the GT before evaluating them by humans. We argue against this, as this is not a real life scenario. An alternative would be to select a subset of X examples for every dataset where the answer was predicted correctly, as was done by Park et al. The issue with this is that we would introduce a bias by choosing the type of examples that were answered correctly, which could e.g. be easier and this would not enable a fair comparison. We could take a subset of examples where the answer was correct for all the models, but this would still not allow future methods to reuse our benchmark and compare results.

\section{Hyperparameters}

\section{removed examples}
